# Supplementary material for: B-cos Networks: Alignment is All We Need for Interpretability
Source: arXiv:2205.10268 source file (2022-05-20)
Supplement: Supplementary file 1 [file b-ablation.tex]

\begin{figure}
    \centering
    \begin{subfigure}[b]{\linewidth}\centering
    \begin{subfigure}[b]{0.155\linewidth}
    \includegraphics[width=\linewidth, trim=1em .5em .5em 0, clip]{supplement/resources/c10-images/C10-Image_99.pdf}
    \end{subfigure}
    \begin{subfigure}[b]{0.155\linewidth}
    \includegraphics[width=\linewidth, trim=1em .5em .5em 0, clip]{supplement/resources/c10-images/C10-Image_99-B_1.0.pdf}
    \end{subfigure}
    \begin{subfigure}[b]{0.155\linewidth}
    \includegraphics[width=\linewidth, trim=1em .5em .5em 0, clip]{supplement/resources/c10-images/C10-Image_99-B_1.25.pdf}
    \end{subfigure}
    \begin{subfigure}[b]{0.155\linewidth}
    \includegraphics[width=\linewidth, trim=1em .5em .5em 0, clip]{supplement/resources/c10-images/C10-Image_99-B_1.5.pdf}
    \end{subfigure}
    \begin{subfigure}[b]{0.155\linewidth}
    \includegraphics[width=\linewidth, trim=1em .5em .5em 0, clip]{supplement/resources/c10-images/C10-Image_99-B_2.0.pdf}
    \end{subfigure}
    \begin{subfigure}[b]{0.155\linewidth}
    \includegraphics[width=\linewidth, trim=1em .5em .5em 0, clip]{supplement/resources/c10-images/C10-Image_99-B_2.5.pdf}
    \end{subfigure}
    \end{subfigure}
    \begin{subfigure}[b]{\linewidth}\centering
    \begin{subfigure}[b]{0.155\linewidth}
    \includegraphics[width=\linewidth, trim=1em .5em .5em 0, clip]{supplement/resources/c10-images/C10-Image_122.pdf}
    \end{subfigure}
    \begin{subfigure}[b]{0.155\linewidth}
    \includegraphics[width=\linewidth, trim=1em .5em .5em 0, clip]{supplement/resources/c10-images/C10-Image_122-B_1.0.pdf}
    \end{subfigure}
    \begin{subfigure}[b]{0.155\linewidth}
    \includegraphics[width=\linewidth, trim=1em .5em .5em 0, clip]{supplement/resources/c10-images/C10-Image_122-B_1.25.pdf}
    \end{subfigure}
    \begin{subfigure}[b]{0.155\linewidth}
    \includegraphics[width=\linewidth, trim=1em .5em .5em 0, clip]{supplement/resources/c10-images/C10-Image_122-B_1.5.pdf}
    \end{subfigure}
    \begin{subfigure}[b]{0.155\linewidth}
    \includegraphics[width=\linewidth, trim=1em .5em .5em 0, clip]{supplement/resources/c10-images/C10-Image_122-B_2.0.pdf}
    \end{subfigure}
    \begin{subfigure}[b]{0.155\linewidth}
    \includegraphics[width=\linewidth, trim=1em .5em .5em 0, clip]{supplement/resources/c10-images/C10-Image_122-B_2.5.pdf}
    \end{subfigure}
    \end{subfigure}
    % \vspace{-1.75em}
    \caption{
    \textbf{Column 1}: Input images.
    \textbf{Columns 2-6}: Corresponding explanations for `horse' and `car' of models trained with increasing (left to right) values of B$\in$%
$\{1, 1.25, 1.5, 2, 2.5\}$. 
    With higher B, the linear transformations $\mat w_{1\rightarrow l}$ become more interpretable.
    }
    \label{fig:b-abl-quali}
    % \vspace{-1em}
\end{figure}
