# Supplementary material for: B-cos Networks: Alignment is All We Need for Interpretability
Source: arXiv:2205.10268 source file (2022-05-20)
Supplement: Supplementary file 11 [file param_ablation.tex]

% \begin{table}
    \centering
    {\setlength{\tabcolsep}{0.25em}\setlength\extrarowheight{-1pt}
    \begin{tabular}{|>{\centering\arraybackslash}  >{\centering\arraybackslash}p{1.85cm} |
    >{\centering\arraybackslash}p{.6cm} |
    >{\centering\arraybackslash}p{.6cm} |
    >{\centering\arraybackslash}p{.6cm} |
    >{\centering\arraybackslash}p{.6cm} |
    >{\centering\arraybackslash}p{.6cm} |
    >{\centering\arraybackslash}p{.6cm} |
    >{\centering\arraybackslash}p{.6cm} |
    >{\centering\arraybackslash}p{.6cm} |
    }
    \cline{2-9}
    % \hline
    % \footnotesize \textbf{Model} 
%   \footnotesize \bf Model type$\,\rightarrow$ 
    \multicolumn{1}{c}{} &\multicolumn{8}{|c|}{\footnotesize \bf \bcos{} DenseNet-121 models}
    \\\hline
  \multicolumn{1}{|c|}{\footnotesize \bf MaxOut}&\footnotesize \bf no &\multicolumn{7}{c|}{\footnotesize \bf Maxout with 2 units}
    \\\hline
    \footnotesize \textbf{g-factor}
    & {\footnotesize 32}
    & {\footnotesize 20}
    & {\footnotesize 22}
    & {\footnotesize 24}
    & {\footnotesize 26}
    & {\footnotesize 28}
    & {\footnotesize 30}
    & {\footnotesize 32}
    \\\hline
    \footnotesize \textbf{\#Params.~(M)}
    & {\footnotesize 7.9}
    & {\footnotesize 6.8}
    & {\footnotesize 8.0}
    & {\footnotesize 9.4}
    & {\footnotesize 10.8}
    & {\footnotesize 12.4}
    & {\footnotesize 14.0}
    & {\footnotesize 15.8}
    \\\hline
    \footnotesize \textbf{Accuracy (\%)}
    &\footnotesize 72.6 % single maxout
    &\footnotesize 72.8 % G=20
    &\footnotesize 73.2 % G=22
    &\footnotesize 73.6 % G=24
    &\footnotesize 73.7 % G=26
    &\footnotesize 74.0 % G=28
    &\footnotesize 73.9 % G=30
    &\footnotesize 74.3 % G=32
    \\\thickhline
    \multicolumn{9}{c}{\footnotesize }
    \\\hline
    \multicolumn{9}{|c|}{\footnotesize {\bf Standard DenseNet-121:} accuracy 74.4; parameters 7.9; g-factor 32}
    \\\hline
    \end{tabular}}
