# Supplementary material for: B-cos Networks: Alignment is All We Need for Interpretability
Source: arXiv:2205.10268 source file (2022-05-20)
Supplement: Supplementary file 13 [file 0.0-packages_and_commands.tex]

%%%%%%%%%%%%%%
%% PACKAGES %%
%%%%%%%%%%%%%%
\usepackage{times}
\usepackage{epsfig}
\usepackage{graphicx}
\usepackage{amsmath}
\usepackage{mathtools}
\usepackage{amssymb}
\usepackage{pifont}% http://ctan.org/pkg/pifont
\newcommand{\cmark}{\ding{51}}%
\newcommand{\xmark}{\ding{55}}%
\usepackage{subcaption}
\usepackage{wrapfig}
\usepackage{multirow}
\usepackage{amsthm}
\usepackage{changepage}

\usepackage{floatrow}
% Table float box with bottom caption, box width adjusted to content
\newfloatcommand{capbtabbox}{table}[][\FBwidth]

% \usepackage{xr} %Cross-referencing to main paper
% \usepackage{xr-hyper}
\usepackage{algorithm2e,setspace}
\usepackage[document]{ragged2e}
\usepackage{parskip}
\usepackage{array}
\usepackage{enumitem}       % enumerations
\usepackage{caption}
\captionsetup{font=small}


\usepackage{xcolor}
\usepackage[pagebackref=true,breaklinks=true,colorlinks,bookmarks=false]{hyperref}



\usepackage[capitalize]{cleveref}
\crefname{section}{Sec.}{Secs.}
\Crefname{section}{Section}{Sections}
\Crefname{table}{Table}{Tables}
\crefname{table}{Tab.}{Tabs.}
\renewcommand{\figurename}{Fig.}
\renewcommand{\tablename}{Tab.}
\makeatletter
\renewcommand\@bibitem[1]{\item\if@filesw \immediate\write\@auxout
    {\string\bibcite{#1}{S\the\value{\@listctr}}}\fi\ignorespaces}% <------------
\def\@biblabel#1{[S#1]}% <-------------------
\makeatother


\newlength{\thickarrayrulewidth}
\setlength{\thickarrayrulewidth}{2\arrayrulewidth}

\makeatletter
\def\thickhline{%
  \noalign{\ifnum0=`}\fi\hrule \@height \thickarrayrulewidth \futurelet
   \reserved@a\@xthickhline}
\def\@xthickhline{\ifx\reserved@a\thickhline
               \vskip\doublerulesep
               \vskip-\thickarrayrulewidth
             \fi
      \ifnum0=`{\fi}}
\makeatother

% Indentation
\setlength{\parindent}{1.25em}
\setlength{\parskip}{.2em}
 \def\baselinestretch{1}


%%%%%%%%% PAPER ID  - PLEASE UPDATE
\def\cvprPaperID{6365} % *** Enter the CVPR Paper ID here
\def\confName{CVPR}
\def\confYear{2022}

%%%%%%%%%%%%%%
%% COMMANDS %%
%%%%%%%%%%%%%%
\newcommand{\bcos}{B-cos}

\newcommand{\colornum}[1]{{\textbf{\color[RGB]{39, 158, 206}#1}}}
\newcommand{\mat}[1]{\MakeUppercase{\mathbf{#1}}}
\renewcommand{\vec}[1]{\MakeLowercase{\mathbf{#1}}}
\newcommand{\tmat}[1]{$\mat{#1}$}
\newcommand{\vmat}[1]{$\vec{#1}$}
\newcommand{\putfig}{} % As a dummy until defined.
\newcommand\myeq{\mkern1.25mu{=}\mkern1.25mu}
\newcommand\myminus{\mkern1.25mu{-}\mkern1.25mu}

\newcommand{\myparagraph}[2][0]{\vspace{#1em}\noindent{\bf #2}}


\newboolean{showcomments}
\setboolean{showcomments}{false}


\numberwithin{equation}{section}
\numberwithin{figure}{section}
\numberwithin{table}{section}
\renewcommand{\thefigure}{\thesection\arabic{figure}}
\renewcommand{\thetable}{\thesection\arabic{table}}
